# Supplementary material for: HiPrompt: Few-Shot Biomedical Knowledge Fusion via Hierarchy-Oriented Prompting
Source: arXiv:2304.05973 source file (2023-04-12)
Supplement: Supplementary file 1 [file appendix.tex]

\section*{Appendix}

\section{App 1. Test}
\label{appx:benchmark}
